# Supplementary material for: Machine learning for a finite size correction in periodic coupled cluster theory calculations
Source: arXiv:2204.00092 source file (2022-03-31)
Supplement: Supplementary file 1 [file SI.pdf]

# Supplementary Material for "Machine learning for a finite size correction in periodic coupled cluster theory calculations"

Laura Weiler,[1] Tina N Mihm,[1] and James J. Shepherd[1, a)]

*Department of Chemistry, University of Iowa*

(Dated: March 30, 2022)

## I. STRUCTURE FACTOR PREPROCESSING AND THERMODYNAMIC LIMIT EXTRAPOLATIONS

We preprocess the raw $\mathbf{G}$ and $S_{\mathbf{G}}$ attained from our uegccd and VASP codes in order to fit the structure factor to a 1D function in $|\mathbf{G}| = G$ using the following averaging scheme:

$$\overline{S_G} = \frac{\sum_{|\mathbf{G}|=G} S_{\mathbf{G}}}{N_G} \tag{1}$$

Where $N_G$ is the number of momentum transfers computed as $N_G = \sum_{|\mathbf{G}|=G} 1$. For Na and Li, VASP projects $S_{\mathbf{G}}$ onto UEG-like grids which allows us to use the same averaging scheme. $\overline{S_G}$ is then scaled by $1/N$ for the UEG and $N_k$ for Li and Na in order for the units in the correlation energy sum to work out to Ha/el for the UEG and eV/unit cell for the real systems. Here, $N$ is the total number of electrons and $N_k$ is the total number of grid points. The VASP $G$ values are also scaled from units of $\text{Å}^{-1}$ to a.u. in order to match the UEG units.

Once the structure factor has been preprocessed using the averaging and scaling procedure described above, GPR models are trained on $G$, $\overline{S_G}$ pairs. From the trained GPR models we obtain a continuous representation of the 1D structure factor as a function of momentum transfer vector magnitudes: $S(G)$.

To find the energy, the $S(G)$ first needs to be projected onto finite grids which can then be extrapolated over in the same manner as the original CCSD correlation energy estimates. GPR is used to project $S(G)$ onto a grid of $G$s from the UEG, applying scale factors to account for the particle number and basis set cutoff. Then this rediscretized $S_G^{\mathrm{GPR}}$ is used to calculate the energy using a slightly modified Eq. 2 from the paper:

$$E_{\mathrm{corr}} = \frac{1}{2} \sum_G{}^{\prime} S_G^{\mathrm{GPR}} V_G N_G \tag{2}$$

Where all quantities have been reduced to functions of $G$ and $N_G$ has been introduced to the sum to account for the structure factor averaging.

Once the above steps have been taken such that each GPR model has been used to predict the correlation energy at each grid size for the relevant system, the correlation energy predictions are extrapolated to the thermodynamic limit to attain a bulk CCSD correlation energy prediction. Extrapolations are performed by taking a linear fit over the largest grid sizes' correlation energy predictions to zero on a $N^{-1}$ plot (or $N_k^{-1}$ for Li and Na). For Li and Na, the largest two grids ($3 \times 3 \times 3$ and $4 \times 4 \times 4$) are used for extrapolation. For the UEG, the largest four grids are used for the extrapolation due to the larger range of grid sizes available.

Figure 1 shows the complete extrapolation procedure for Li, Na and the UEG. The black points in Fig. 1 are the original CCSD correlation energies at each grid size, and the black line is the extrapolated CCSD. Li additionally has red x markers for CCSD-FS points whose extrapolation is plotted as a red line. The GPR correlation energy predictions (from Eq. (2)) are plotted as colored triangles, and the extrapolated CCSD-GPR result are colored lines. The colors correspond to the grid size on which the GPR model was trained which was used to generate the CCSD-GPR predictions. A colored, dotted line is included for convenience to show the domain of the extrapolation and to illustrate the slope and intercept of the fit. The solid, horizontal colored lines correspond to the turquoise triangles in Fig. 2 of the main paper and are discussed in detail in the Results section. All extrapolations are performed using the `scipy.optimize.curve_fit` method in the python programming language.

Table I. Differences between CCSD and GPR-predicted energies at a given grid size are provided in order to illustrate how GPR fit error (as provided in Section VI of the paper) affects energy predictions. A negative difference indicates that the original CCSD energy was more negative than the GPR predicted energy.

| System | System size | $\Delta E_{\mathrm{corr}}$ |
|---|---|---|
| Li | 2x2x2 | 3.08E-05 (eV/unit cell) |
| Li | 3x3x3 | -0.00270 (eV/unit cell) |
| Li | 4x4x4 | 0.000425 (eV/unit cell) |
| Na | 2x2x2 | 0.000278 (eV/unit cell) |
| Na | 3x3x3 | -0.000384 (eV/unit cell) |
| Na | 4x4x4 | 0.000153 (eV/unit cell) |
| UEG | N=38 | -0.00292 (Ha/el) |
| UEG | N=54 | -0.00194 (Ha/el) |
| UEG | N=114 | 0.00262 (Ha/el) |
| UEG | N=186 | -0.000716 (Ha/el) |
| UEG | N=294 | 0.00246 (Ha/el) |
| UEG | N=342 | 8.79E-05 (Ha/el) |

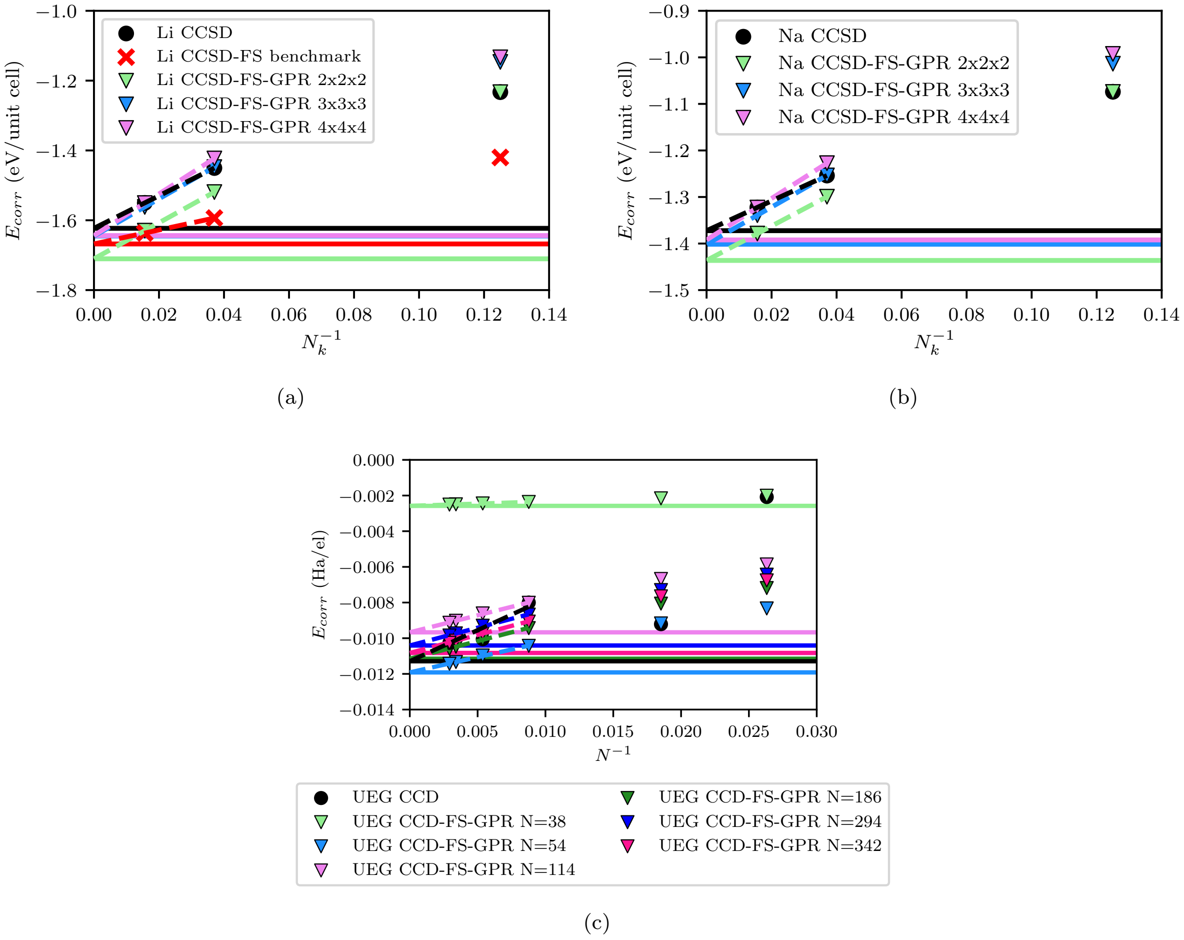


Figure 1. CCSD-GPR TDL extrapolations for: (a) Li bcc, (b) Na bcc, and (c) UEG $r_S = 5$.

[a] Electronic mail: james-shepherd@uiowa.edu
